# Supplementary material for: From Linear to Nonlinear Responses of Thermal Pure Quantum States
Source: arXiv:1806.02054 source file (2018-11-25)
Supplement: Supplementary file 1 [file supple20181024.pdf]

# From Linear to Nonlinear Responses of Thermal Pure Quantum States: *Supplemental Material*

Hiroyuki Endo,[1] Chisa Hotta,[1,*] and Akira Shimizu[1,2,†]

[1]*Department of Basic Science, The University of Tokyo, 3-8-1 Komaba, Meguro, Tokyo 153-8902, Japan*
[2]*Komaba Institute for Science, The University of Tokyo, 3-8-1 Komaba, Meguro, Tokyo 153-8902, Japan*
(Dated: October 24, 2018)

## A. Necessary condition (iii) in the limit of infinitesimal external field

Among the three necessary conditions for the applicability of our theory, condition (iii) is the most nontrivial one. This condition is reasonable in the sense that, in the limit of $h \to 0$, it reduces to the corresponding condition for the linear response (LR) theory (i.e., the Kubo formula) [1–3]. Unfortunately, the latter condition for the LR does not seem recognized widely, despite its importance. We therefore present it briefly in this supplemental section.

We here take, as an example, the magnetic susceptibility to a uniform magnetic field. In this case, the system has an equilibrium state at $\omega = 0$, with the Hamiltonian $\hat{H} - h\hat{M}$. Hence, one can check the validity of the Kubo formula by comparing its result with the results of equilibrium statistical mechanics and thermodynamics.

According to thermodynamics, the isothermal susceptibility $\chi_T$ takes a different value from the adiabatic susceptibility $\chi_S$. They are related by

$$\chi_S = \chi_T - \frac{T}{c_h}\left[\left(\frac{\partial m}{\partial T}\right)_h\right]^2, \tag{S1}$$

where $m := M/N$, and $c_h$ is the specific heat at a constant magnetic field. Therefore,

$$\chi_T \geq \chi_S, \tag{S2}$$

and the equality holds only at the first-order phase transition (where $c_h \to \infty$) or in a nonmagnetic phase at $h = 0$ (for which $m = 0$).

Experimental results should agree with either $\chi_T$ or $\chi_S$ or another thermodynamic susceptibility, depending on the experimental conditions. Then, a question arises: Does either one of $\chi_T$ or $\chi_S$ (or another thermodynamic one) agree with $\chi_{\rm K}$? Here, $\chi_{\rm K}$ is the $\omega \to 0$ limit of the susceptibility obtained by the Kubo formula.

As an answer to this nontrivial question, Kubo showed in Ref. [1] that $\chi_{\rm K} = \chi_T$ *if and only if* Eq.(3.26) of [1] is satisfied. (See also Refs. [2, 3].)

Condition (iii) of the present theory is a natural generalization of this requirement to the nonlinear nonequilibrium regime.

## B. Low energy effective model for the ferromagnetic Heisenberg chain

In the main text, we considered the $S = 1/2$ ferromagnetic Heisenberg chain, and calculated the response functions $\mathrm{Im}\,\chi_{\rm sub}(q, \omega; h)$ based on our formula, Eq.(5).

To capture the microscopic origin of the obtained $\chi$ in Fig. 2, we consider a small subspace that is spanned by the fully polarized, one-magnon, and two-magnon states. Notice that there are low energy excited states with more magnons, while we discard them for simplicity. Figure S1 (b) shows the energy levels of $\hat{H}$ confined in this subspace. The red solid line is the one-magnon dispersion starting from the bottom of the band. This branch is fully absorbed in the magnon continuum indicated as shaded regions. At $N = 16$, the energy levels ($E_m$) are discrete as shown by dots, while with the increasing $N$, it approaches the continuum, as already confirmed in the exact calculation. There is a two-magnon excitation shown in dotted lines that lies below the continuum.

Using the information on these energy levels and the corresponding eigen states, one obtains the LR within the subspace as

$$\begin{aligned}\mathrm{Im}\,\chi_{\rm sub}(q,\omega) = \sum_{n,m} (\pi/NZ)(\mathrm{e}^{-\beta E_n} - \mathrm{e}^{-\beta E_m}) \\ |\langle n|\hat{M}_q|m\rangle|^2 \delta(\omega - (E_m - E_n)),\end{aligned} \tag{S3}$$

where $Z$ is the partition function. The obtained spectra at $\beta = 2$ are shown by the solid lines in Fig. S1 (a), to be compared with the full spectra $\mathrm{Im}\,\chi$ obtained by our protocol (symbols). One can identify the processes showing the largest contributions; the three lowest levels in Fig. S1(b) transfer to the ones separated by $q$, and the transition energies correspond to the location of the main peaks of each of the spectra. The contributions from the states not included in Fig. S1(b) are still missing in $\mathrm{Im}\,\chi_{\rm sub}$, which should be the reason for their dips compared to $\mathrm{Im}\,\chi$. In fact the many-magnon branches goes down to the lowest energy level at $k = 0$ and become all degenerate. Our $\mathrm{Im}\,\chi$ gives the complete profile of response.

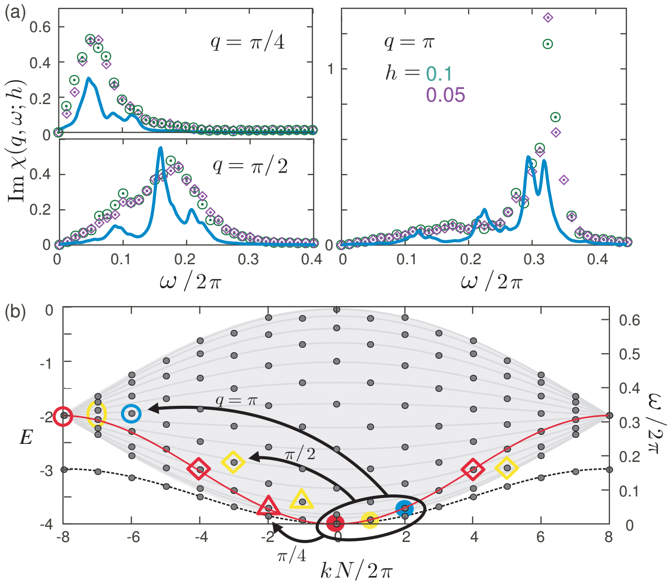


FIG. S1. (a) Comparison of $\mathrm{Im}\,\chi$ in Eq. (5) in the LR regime for $h = 0.05$ (circles) and 0.1(diamonds). Solid lines are $\mathrm{Im}\,\chi_{\mathrm{sub}}$ defined in the text, obtained from the spectrum in panel (b), broadened by the Lorentzian of half-width $\delta\omega = 1/2t_{\mathrm{end}}$. (b) Energy spectrum of the model restricted to the small subspace with up to two magnons. One magnon dispersion (red solid line), bound state of two magnons (dashed line), and the two-magnon continuum (shaded area) are shown together. The processes with large weight on the main peaks of panel (a) are shown for each $q = \pi/4, \pi/2, \pi$ (triangles, rectangles, open circles) starting from the three lowest energy levels (filled circles). The energy differences correspond to the peak positions.

## C. Supporting results for the kagome antiferromagnet

The time evolution of the $S = 1/2$ kagome antiferromagnet at $h = 0.5$ in the nonlinear regime is shown in Fig. S2 (a), which gives $\chi(\boldsymbol{q}, \omega; h)$ in Fig. 3(b) of the main text. Each thin line gives the time evolution starting from different initial cTPQ states, and their average is shown in broken line. The sample dependence is very small where we averaged over three samples for $\chi(q, \omega; h)$. A good convergence should be supported by the large entropy (inset of Fig. 3(b)) that is further enhanced by $h$. The asterisk symbol in inset of Fig. 3(b) indicates the energy density of the system after the quench.

We show in Fig. S2(b) the comparison of the spectrum at $h = 0.02$ and 0.05 for $k_BT = 0.1$. A good agreement shows that the system is in the linear response regime at this field strength, as in the case of ferromagnetic Heisenberg chain.

In finite cluster calculation of a two dimension, the finite size effect including the artifact due to small system size as well as the choice of the shape of the cluster may alter the result. However, in a kagome lattice antiferromagnet, quite large numbers of excited states consist of magnons that localize in space due to kinetic frustration effect [4]. In fact, as shown in Fig. S2(c), the finite size effect of the spectrum we obtained reveals as a spike, reflecting the small number of levels due to the former effect. However, the oscillation center of the spikes shows good consistency with the smooth curve at $N = 27$, indicating that the feature of the spectrum is well preserved even in a system size as small as $N = 18$. Thus, already at $N = 27$ we find a smooth spectrum that does not alter the essential feature of the true bulk spectrum.

* chisa@phys.c.u-tokyo.ac.jp
† shmz@as.c.u-tokyo.ac.jp

[1] R. Kubo, J. Phys. Soc. Jpn. **12**, 570 (1957).
[2] R. Kubo, M. Toda, and N. Hashitsume, *Statistical Physics II: Nonequilibrium Statistical Mechanics* (Springer-Verlag, Berlin, 1985).
[3] A. Shimizu and H. Kato, *Nonequilibrium Mesoscopic Conductors Driven by Reservoirs, Low-Dimensional Systems — Interactions and Transport Properties* [ed. T. Brandes], Lecture Notes in Physics 54, pp.3-22 (Springer, 2000); arXiv:cond-mat/9911333.
[4] X. Plat, T. Momoi, C. Hotta, Phys. Rev. B **98**, 014415 (2018).

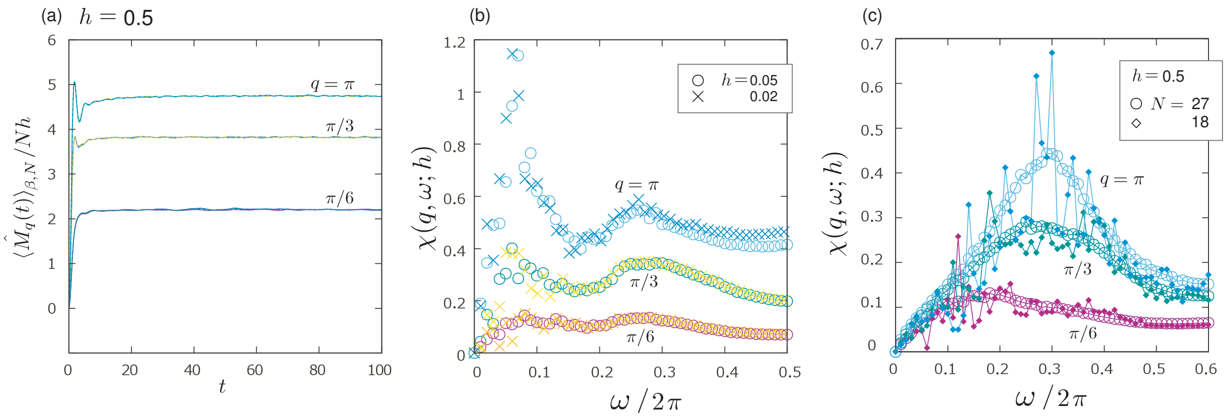


FIG. S2. Supporting results of the spin-1/2 kagome antiferromagnet at $N = 27$. (a) Time evolution of $\langle M_q(t) \rangle$ that yields the nonlinear response (Fig. 3(b)) at $h = 0.5$ and $k_B T = 0.1$. The solid lines give the results starting from different TPQ states, and the broken lines are their averages. (b) Comparison of $\chi(q, \omega; h)$ between $h = 0.02$ and 0.05 at $k_B T = 0.1$. The latter is the same as given in Fig. 3(a). A somewhat oscillating deviation of $h = 0.02$ at small $\omega$ dissolves when taking an average of many samples (while here, we take three sample averages for all data in this figure). (c) Comparison of $\chi(q, \omega; h)$ at $h = 0.5$ between $N = 27$ and 18. The spikes found in $N = 18$ data is due to the small system size which is smoothed out already at $N = 27$.
